# Supplementary material for: Opto-electronic properties and solar cell efficiency modelling of Cu$_2$ZnXS$_4$ (X=Sn,Ge,Si) kesterites
Source: arXiv:2011.12764 source file (2020-11-25)
Supplement: Supplementary file 1 [file Supplementary_Material.pdf]

## Supplementary Materials

### S1. Optical properties

The optical properties have been obtained through the calculation of the dielectric tensor  $\epsilon = \epsilon_1 + i\epsilon_2$  scaled by the vacuum electrical permittivity  $\epsilon_0$ . The imaginary part  $\epsilon_2(E)$  has been obtained via the application of the Fermi golden rule, i. e., the summation over the possible transitions between filled states in the valence band and empty states in the conduction band for various  $\mathbf{k}$ -points as presented in Eq. (S1) and implemented in VASP as described in [S1].

$$\epsilon_2(E) = \left( \frac{4\pi}{|\mathbf{E}(\omega)|} \right)^2 \sum_{c,v,\mathbf{k}} |\langle c_{\mathbf{k}} | \mathcal{H}_{\text{er}} | v_{\mathbf{k}} \rangle|^2 \delta(E_{c,\mathbf{k}} - E_{v,\mathbf{k}} - E), \quad (\text{S1})$$

The summation is realised over the valence and conduction band energy levels  $v, c$  for a given  $\mathbf{k}$ -point  $\mathbf{k}$ .  $E$  is the photon energy ( $\hbar\omega$ ) and  $\mathcal{H}_{\text{er}}$  is the electron-radiation interaction Hamiltonian. Finally,  $\mathbf{E}(\omega)$  is the external perturbation applied. The real part of the dielectric tensor  $\epsilon_1(E)$  is obtained via the Kramers-Kronig transformation implemented in VASP as described in [S1] and presented in Eq. (S2).

$$\epsilon_1(E) = 1 + \frac{2}{\pi} P \int_0^\infty \frac{\epsilon_2(E') E'}{E'^2 - E^2} dE', \quad (\text{S2})$$

Based on the calculation of the dielectric tensor, various material optical properties can be calculated such as the absorption coefficient  $\alpha(E)$  as presented in Eq. (S4) and calculated based on the extinction coefficient  $\kappa(E)$  (Eq. (S3)).

$$\kappa(E) = \frac{1}{\sqrt{2}} \sqrt{-\epsilon_1(E) + \sqrt{\epsilon_1^2(E) + \epsilon_2^2(E)}} \quad (\text{S3})$$

$$\alpha(E) = \frac{4\pi E \kappa(E)}{hc} \quad (\text{S4})$$

In addition, the materials refractive index  $n(E)$  and reflectivity  $R(E)$  is computed using respectively Eqs. (S5) and (S6).

$$n(E) = \frac{1}{\sqrt{2}} \sqrt{\epsilon_1(E) + \sqrt{\epsilon_1^2(E) + \epsilon_2^2(E)}} \quad (\text{S5})$$

$$R(E) = \frac{(n-1)^2 + \kappa^2}{(n+1)^2 + \kappa^2} \quad (\text{S6})$$

### S2. Electrical power conversion efficiency

Initially in 1960, Shockley and Queisser (SQ) proposed a model entitled "detailed balance limit of efficiency" to assess the theoretical upper limit of a PN-junction solar cell [S2]. This model assumes only radiative recombinations as recombination mechanism for electron-hole pairs (EHPs) and considers the solar cell as a black body (BB) at a given temperature  $T$ . In this case, the theoretical upper efficiency can be expressed as the maximal value of the ratio between the electrical power generated by the solar cell and the solar power as presented in Eq. (S7). With  $V$ , the voltage induced by the generation of EHPs,  $d$ , the absorber layer thickness,  $q$ , the electron charge and  $\Phi_{\text{Sun}}$  the solar spectrum expressed in  $\text{eV}^{-1}\text{m}^{-2}\text{s}^{-1}$ . The SQ model assumes a solar cell with an ideality factor of 1 and an internal

quantum efficiency  $Q_i = 1$  meaning that every photon absorbed generates an EHP which is either collected or re-emitted as a photon contributing to the solar cell black body spectrum (i. e., no non-radiative recombination).

$$\eta = \max_V \left( \frac{J(V, d)V}{q \int_0^\infty E \Phi_{\text{sun}}(E) dE} \right), \quad (\text{S7})$$

with the total current density  $J(V, d)$  (Eq. (S8)) equals to the sum of the short circuit current density  $J_{\text{SC}}$  (Eq. (S9)) and the radiative saturation current density  $J_{\text{rad}}$ . The latter one is presented in Eq. (S10) with  $q$  the electron charge and  $k_B$  the Boltzmann constant.

$$J(V, d) = J_{\text{SC}}(d) + \underbrace{J_{\text{rad},0}(d)(1 - \exp(qV/k_B T))}_{J_{\text{rad}}(d,V)} \quad (\text{S8})$$

The current density under short circuit condition can be expressed as the number of photons absorbed per unit of time. First SQ took as incident photon flux, the BB spectrum at  $T = 6000\text{K}$  [S2]. Then, the product of  $\Phi_{\text{sun}}$  by the absorptance  $A(E)$  results in the number of EHPs generated in the absorber layer and contributing to the short circuit current density. Assuming a Heaviside step function for the absorptance, every photon with an energy  $\hbar\omega > E_G$  is absorbed.

$$J_{\text{SC}}(d) = q \int_{E_G}^\infty A(E, d) \Phi_{\text{sun}}(E) dE \quad (\text{S9})$$

Secondly, the radiative recombination current density term which describes the number of EHP recombinations in a solar cell at temperature  $T$  can be expressed as described in Eq. (S10). In this equation, the radiative recombination rate under equilibrium condition,  $R_{\text{rad},0}(d)$  is described as the integration over the energy of the product between the BB radiation spectrum at a temperature  $T$  and the materials absorptance spectrum (Eq. (S11)).

$$J_{\text{rad},0}(d) = q R_{\text{rad},0}(d) \quad (\text{S10})$$

$$R_{\text{rad},0}(d) = \frac{2\pi}{c^2 h^3} \int_{E_G}^\infty A(E, d) \left[ \exp(E/k_B T) - 1 \right]^{-1} E^2 dE \quad (\text{S11})$$

As a result, the SQ model parameters are the solar cell temperature  $T$  (usually 300 K), the absorber layer thickness  $d$  and the materials bandgap  $E_G$  used to compute the material absorptance. The solar cell is therefore assumed both infinitely thin and infinitely thick. First, infinitely thin, because it is assumed that every EHP generated is either recovered at the electrodes boundaries (i. e., no non-radiative recombination or  $Q_i = 1$ ). And, secondly, infinitely thick, because it is assumed that every photon for which the energy  $\hbar\omega$  is greater than the bandgap energy  $E_G$  will be absorbed (Heaviside step function for the absorptance). A first straightforward improvement of this model is performed by taking the Air Mass 1.5 (AM1.5) photon flux as the emission spectrum of the sun which is commonly used to characterise solar cells under standard conditions. Secondly, using the *ab initio* optical results (i. e., the absorption coefficient  $\alpha(E)$  and the materials reflectivity  $R(E)$ ), the absorptance  $A(E)$  of the absorber layer materials is computed. Assuming a flat solar cell surface and a thin film thickness  $d$ , the Beer-Lambert law is used to calculate the absorptance as expressed in Eq. (S12). A perfect reflection at the rear interface of the solar cell absorber layer is assumed while at the front interface, the material reflectivity  $R(E)$  obtained via first principle calculation is taking into account. In addition, interference effects are neglected.

$$A(E, d) = [1 - R(E)] - \exp(-2\alpha(E)d) \quad (\text{S12})$$

In addition to these improvements, in 2017, Blank *et.al.* proposed an extended detailed balance model via: (i) the use of the internal quantum efficiency  $Q_i$  as model parameter to take into account non-radiative recombinations and (ii) the incorporation of light trapping by taking into account the materials refractive index  $n(E)$  in the calculation of the radiative current density  $J_{\text{rad},0}(n, d)$  [S3]. This refractive index is assumed isotropic which, in this study, is confirmed by the *ab initio* results obtained. (i) First, the internal quantum efficiency is used as a parameter to take into account non-radiative recombinations. As those non-radiative recombinations depend on the presence of defects in the materials acting as recombination centres (intrinsic point defects, grain boundaries, ... *etc.*), it is more convenient in this work, to use this physical quantity as a model parameter. This one is expressed as the ratio between the radiative recombination rate  $R_{\text{rad},0}$  and the total recombination rate:  $R_{\text{rad},0} + R_{\text{nr},0}$ , leading to a non-radiative recombination rate under equilibrium conditions expressed as described in Eq. (S13). This model assumes an identical voltage dependency for the radiative and non-radiative recombination rates.

$$R_{\text{nr},0} = \frac{R_{\text{rad},0}(1 - Q_i)}{Q_i} \quad (\text{S13})$$

(ii) In addition, to take into account the internal reflections and therefore re-absorption in the absorber layer, the Roosbroeck-Shockley equation is used to calculate the radiative recombination current density as described in Eq. (S14). In this one, the absorber layer refractive index  $n(E)$  is injected.

$$J_{\text{rad},0}(d, n) = qp_e(d, E)R_{\text{rad},0}(d, E) = q \frac{\int_{E_G}^{\infty} A(E)\Phi_{\text{BB}}(E)dE}{4d \int_{E_G}^{\infty} n^2(E)\alpha(E)\Phi_{\text{BB}}(E)dE} R_{\text{rad},0}(d, E), \quad (\text{S14})$$

with the BB radiation spectrum described in Eq. (S15).

$$\Phi_{\text{BB}}(E, T) = \frac{2E^2}{h^3 c^2 [\exp(E/k_B T) - 1]} \quad (\text{S15})$$

By implementing these two improvements, the total saturation current density under equilibrium conditions  $J_0(d)$  can be expressed as the sum of the radiative saturation current density  $J_{\text{rad},0}(d)$  and the non-radiative saturation current density  $J_{\text{nr},0}(d)$  obtained via the internal quantum  $Q_i$  efficiency parameter as presented in Eq. (S16).

$$J_0(d) = \frac{J_{\text{rad},0}(1 + (p_e - 1)Q_i)}{p_e Q_i} \quad (\text{S16})$$

Finally, the total current density is obtained using Eq. (.S8). In addition, by injecting the voltage dependent current density  $J(V, d)$  in Eq. (S7), the maximal efficiency is calculated for a given layer thickness  $d$ , at a temperature  $T$  and for an internal quantum efficiency value  $Q_i$ . This one is a function of the absorber materials refractive index  $n(E)$ , absorption coefficient  $\alpha(E)$  and reflectivity  $R(E)$  computed using *ab initio* calculations.

## References

- [S1] M. Gajdoš, K. Hummer, G. Kresse, J. Furthmüller, F. Bechstedt, Linear optical properties in the projector-augmented wave methodology, *Physical Review B* 73 (2006) 045112.
- [S2] W. Shockley, H. J. Queisser, Detailed balance limit of efficiency of p-n junction solar cells, *Journal of Applied Physics* 32 (1961) 510–519.
- [S3] B. Blank, T. Kirchartz, S. Lany, U. Rau, Selection metric for photovoltaic materials screening based on detailed-balance analysis, *Physical Review Applied* 8 (2017) 024032.
